# Supplementary material for: Implicit Autoencoder for Point-Cloud Self-Supervised Representation Learning
Source: arXiv:2201.00785 source file (2023-08-27)
Supplement: Supplementary file 1 [file 07_supp.tex]

%We also try a random cropping strategy instead of cropping the center part. During training, we randomly set the cropping location and we hope the model can detect the missing part successfully. The result shows that it is slightly worse than the center cropping. We think that might because our model is not strong enough to fit this strategy. We show more details in supplementary material.
\setcounter{equation}{8}
\setcounter{figure}{5}

%\section{Supplementary Materials}
We provide additional descriptions of pre-training details in Section~\ref{sec:supp:implement}, and downstream task details in Section~\ref{sec:supp:downstream}. We discuss hypothetical concerns in Section~\ref{sec:supp:discuss}. We present more experiment results and analysis in Section~\ref{sec:supp:result}, and  proof of propositions in Section~\ref{sec:supp:proof}.

\section{Pre-training Details}
\label{sec:supp:implement}
%\subsection{Scene Data Generation}
%Given a point cloud $\mathcal{P}^{\text{gt}}$, we first randomly choose a removing ratio from 0\% to 50\% and apply a center-cropping on it to get the input point cloud  $\mathcal{P}^{\text{in}}$. 
%To build the ground truth label of the implicit function $g_0$(e.g., unsigned distance function), we directly compute the distance $d$ between the query point and nearest point from $\mathcal{P}^{\text{gt}}$. And because the point cloud from the real dataset is usually incomplete, we do not define the sign distance values. 
%For the occupancy value, we set the label to be 1 if the distance $d < 0.005m$, and 0 if $d \geq 0.005m$. 

%\subsection{Pre-training}

\subsection{Scene Data Generation}
To prepare the data for scene-level pre-training, we pre-process the point clouds from ScanNet dataset~\cite{dai2017scannet}. We utilize the sliding window strategy and crop each scene instance into $d \times d \times d$ point cloud cubes, where $d=3.0$ m. Consistent with Qi et al.~\cite{qi2019deep}, we divid the dataset into training (consisting of 8k point clouds) and validation (consisting of 2.6k point clouds) splits. We randomly sub-sample 10,000 points from each point cloud to use as input to the encoder.

Given the lack of high-quality water-tight meshes, we employ the k-nearest neighbor (KNN) strategy~\cite{peterson2009k} to calculate ground-truth unsigned distance functions. Specifically, for each sample point $\mathbf{x}$, we use the KNN algorithm to find the three nearest points from the point cloud and calculate the average distance as the unsigned distance value.

\subsection{Decoder Details}

As mentioned in Section 4.2 of the main body, the IAE encoder maps a given point cloud into a high-dimensional code, and the decoder fits an implicit function that converts the latent code and a query point to an implicit function value. We explore two different designs for the decoder: the Occupancy Network style~\cite{mescheder2019occupancy} and the Convolutional Occupancy Network style~\cite{peng2020convolutional}.

\noindent\textbf{Occupancy Network style:} We use a fully-connected neural network with five ResNet blocks to implement the decoder, taking the latent code from the encoder and the sample point $\mathbf{x}$ as input. For detailed information, please refer to~\cite{mescheder2019occupancy}.

\noindent\textbf{Convolutional Occupancy Network style:} First, we decode the latent code from the encoder to a volumetric feature representation. Then, we use trilinear interpolation to obtain the feature of the sample point $\mathbf{x}$. Next, we use a small fully-connected occupancy network to predict the implicit function value, which comprises multiple ResNet blocks. Please refer to~\cite{peng2020convolutional} for further details.

\subsection{Training Details}
\label{sec:supp_trainingdetails}
We implement all models in PyTorch and use the Adam optimizer without weight decay. The learning rate is set to $10^{-4}$ for all datasets. We use standard data augmentation techniques proposed by~\cite{yang2018foldingnet} for both ShapeNet and ScanNet pre-training. For ShapeNet, we pre-train the models for 600 epochs. For ScanNet, we pre-train the models for 1,000 epochs.

\section{Downstream Task Details}
\label{sec:supp:downstream}

After pre-training, the pre-trained encoder is transferred to downstream tasks.

\subsection{Shape Classification}

We respectively sample 1,024 and 2,048 points from each 3D shape in ModelNet40~\cite{wu20153d} and ScanObjectNN~\cite{uy2019revisiting} and utilize the 3-channel coordinates as input. The same training settings are adopted for the two datasets. For the DGCNN~\cite{wang2019dynamic} backbone, we fine-tune the network for 200 epochs with a batch size of 32 and set the learning rate as $1 \times 10^{-3}$ with a weight decay of $5 \times 10^{-1}$. For the M2AE~\cite{zhang2022point} backbone, we fine-tune the network for 300 epochs with a batch size of 32 and set the learning rate as $5 \times 10^{-4}$ with a weight decay of $5 \times 10^{-2}$. 

\subsection{3D Object Detection}
We replicate the settings used in the original paper. To train VoteNet~\cite{qi2019deep}, we fine-tune the network using an Adam optimizer with a batch size of 8 and an initial learning rate of 0.001. After 80 epochs, we reduce the learning rate by a factor of 10 and then again by another factor of 10 after 120 epochs.

To train CAGroup3D~\cite{wang2022cagroup3d} on both ScanNet and SUN RGB-D datasets, we set the batch size, initial learning rate, and weight decay to 16, 0.001, and 0.0001, respectively. For ScanNet, we fine-tune for 120 epochs and reduce the learning rate by a factor of 10 at the 80$^\text{th}$ epoch and again at the 110$^\text{th}$ epochs. For SUN RGB-D, we fine-tune for 48 epochs and reduce the learning rate at the 32$^\text{th}$ and the 44$^\text{th}$ epochs.

\subsection{Indoor 3D Semantic Segmentation}

We present the evaluation of our model on the S3DIS dataset using 6-fold cross-validation~\cite{armeni20163d}. We replicate the settings in the original paper for consistency.

To train the DGCNN model, we adopt a batch size of 32 and an initial learning rate of $1 \times 10^{-1}$ using a stochastic gradient descent optimizer. We reduce the learning rate gradually until it reaches 0.001 using cosine annealing.

For the PointNeXt~\cite{qian2022pointnext} model, we select the PointNeXt-XL version and fine-tune it with an AdamW optimizer, where the weight decay is 10$^{-4}$, the initial learning rate is 0.001, and the batch size is 32. We use the cosine annealing method to reduce the learning rate during training.

\begin{figure}[t]
    \centering
    \includegraphics[width=\columnwidth]{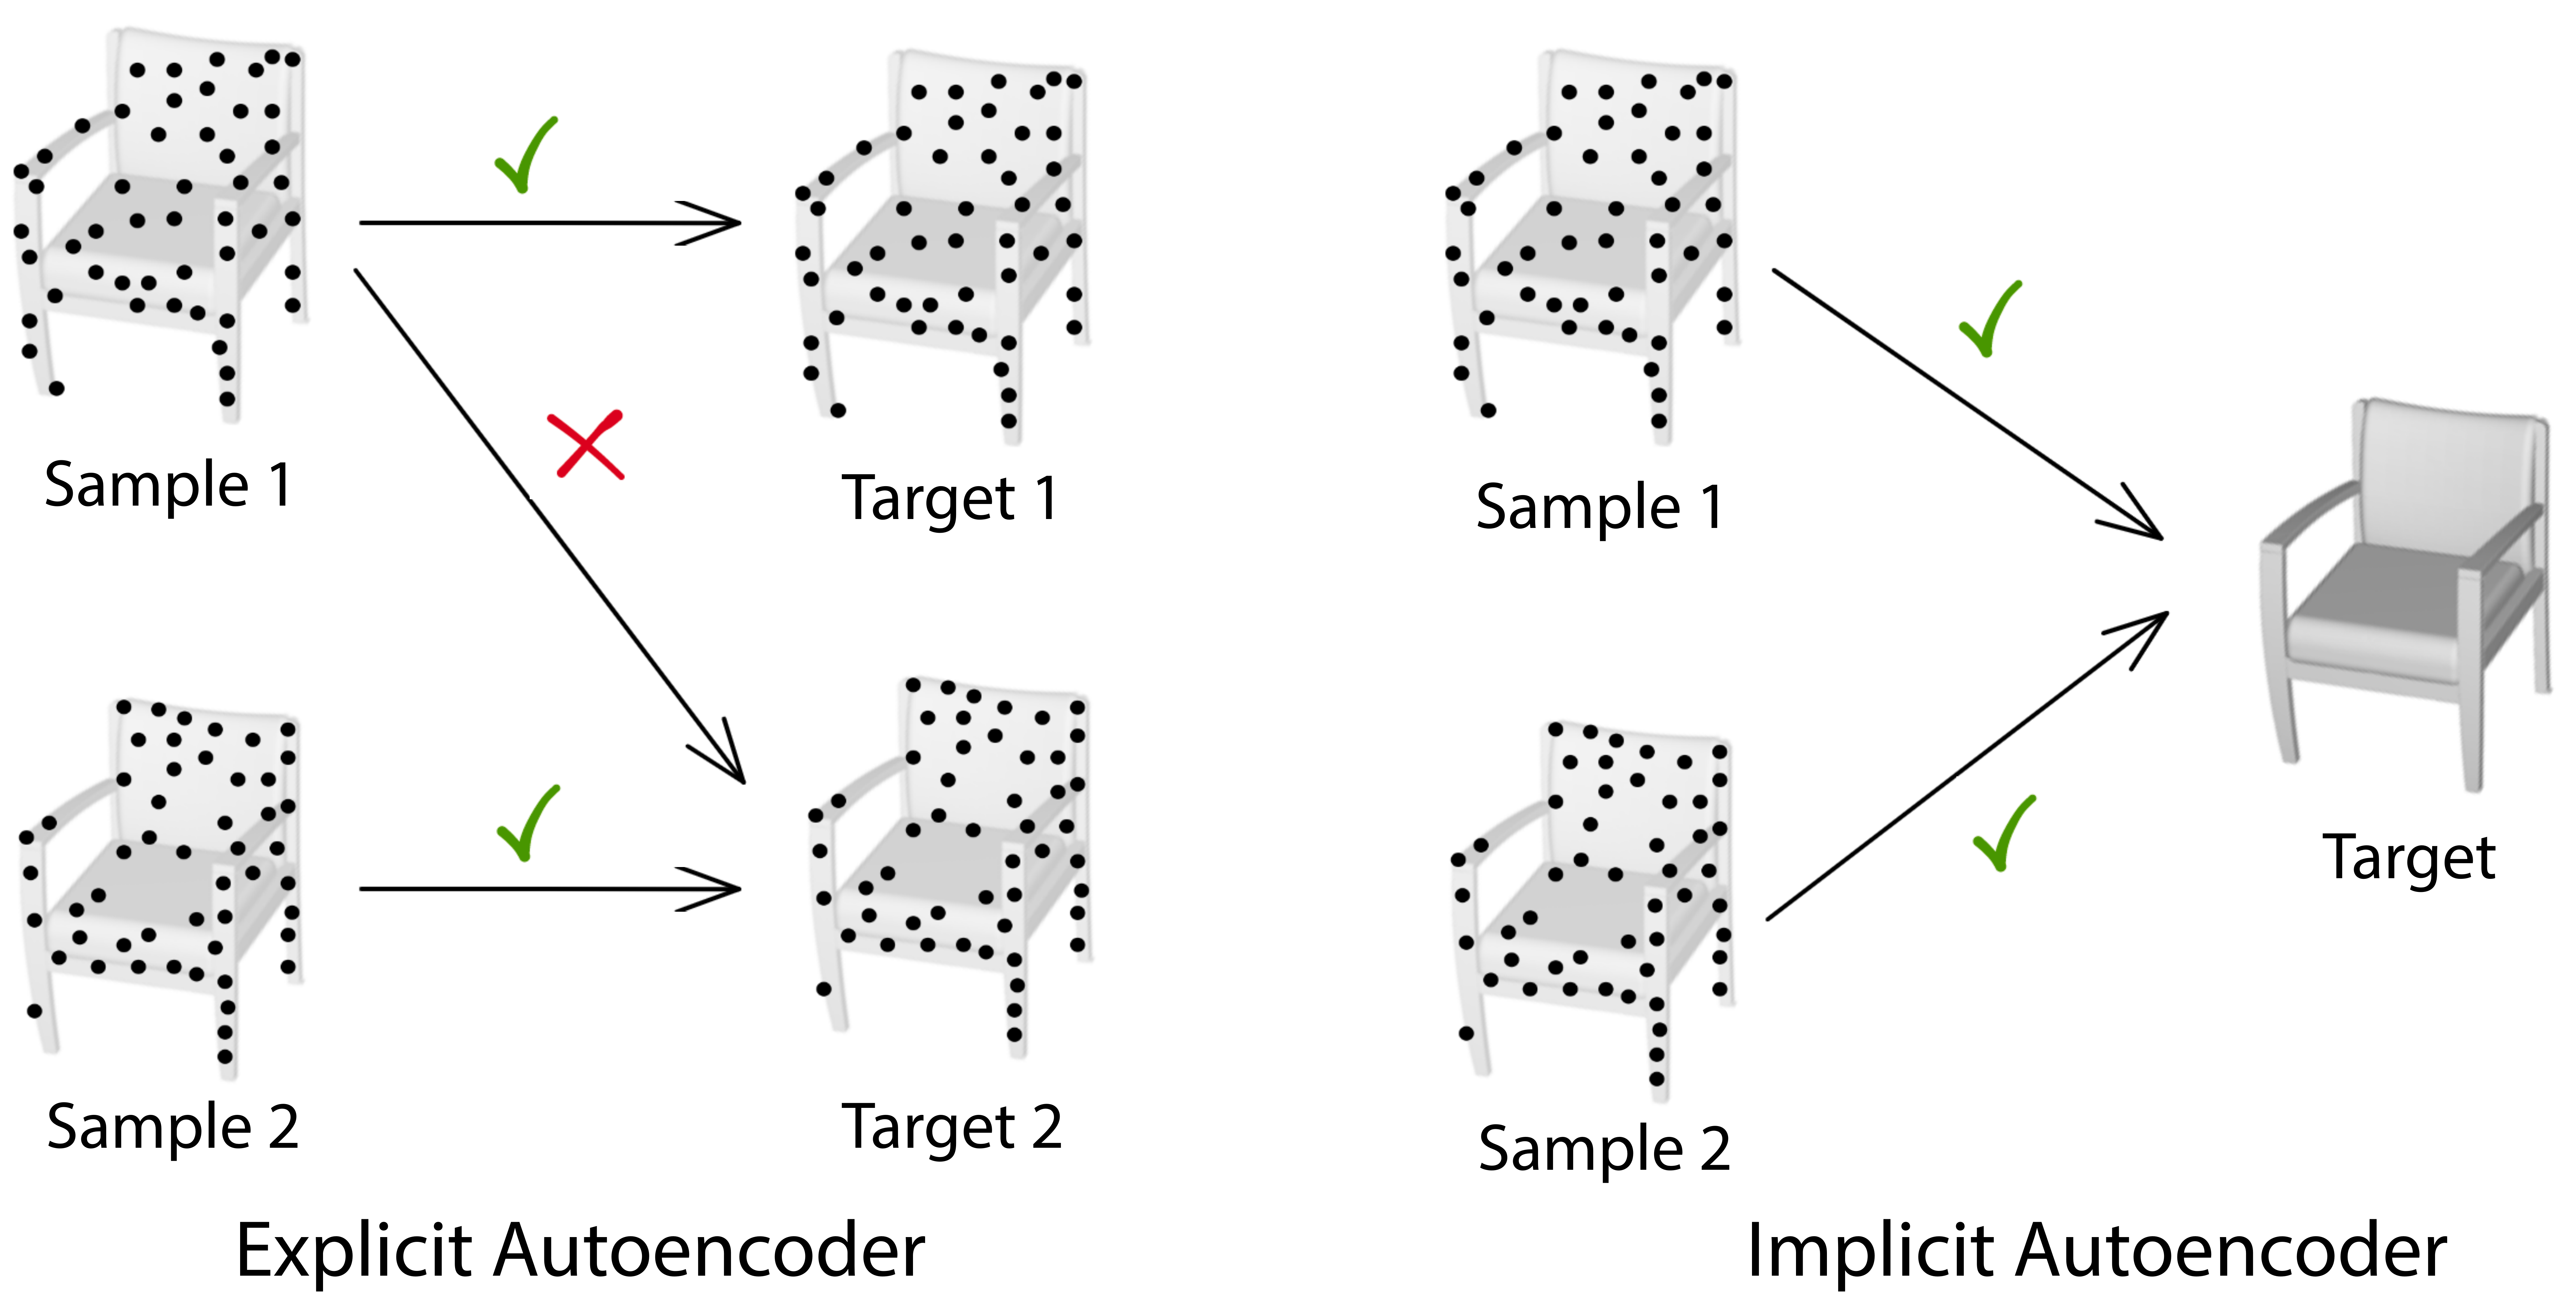}
    \caption{\small{\textbf{Comparison between Explicit Autoencoder and Implicit Autoencoder}. Given a 3D shape, we randomly take two samples. For Implicit Autoencoder, we use 3D CAD model to represent the implicit function target for better visualization.}}
    \label{fig:supp_compare}
    \vspace{-10pt}
\end{figure}
\section{Discussion}
\label{sec:supp:discuss}

\subsection{What is the difference between data augmentation and sampling variation?}

Sampling variation refers to the fact that different point cloud samples of the same 3D shape contain different noises induced from various sources, such as intrinsic noises from sensors and interference from the environment. In the explicit autoencoding paradigm, the encoder is required to encode not only the 3D geometry but also information about the specific discrete sampling of the 3D shape into the latent code, which can lead to sampling variation. This is because the decoder must reconstruct a point cloud that matches the original point cloud perfectly. For example, as shown in Figure~\ref{fig:supp_compare}, given a 3D shape and two randomly selected samples, the explicit autoencoder forces the decoder to output the same sample as the input. If the target sample changes, the loss increases due to incorrect mapping, even though the different samples represent the same shape. Thus, the explicit autoencoding paradigm must learn the mapping that includes sampling variation. In contrast, the implicit autoencoder does not face this problem because different samples map to the same target, which is the implicit representation of the 3D shape.

Data augmentation is a standard technique for point-cloud learning, including rotation, translation, scaling, and sub-sampling. As mentioned in the supplement's Section~\ref{sec:supp_trainingdetails}, IAE uses all of these standard data augmentation methods during pre-training, as other approaches do. For instance, IAE uses different sub-samples of the same 3D shape as input, but all of these sub-samples share the same target, which is the implicit function of the 3D shape.

\subsection{Is it a fair comparison with existing self-supervised learning approaches?}

In this subsection, we discuss the fairness of the comparison between the Implicit Autoencoder (IAE) and existing self-supervised learning approaches. Our approach differs from existing methods in that we use dense point clouds (50k points) or mesh data from ShapeNet to generate the implicit function label, while existing approaches utilize sparse, sub-sampled point clouds (i.e., 1k $\sim$ 2k points) for pre-training. We argue that the point of pre-training is to extract as much information as possible from all available data. Therefore, it is natural to include dense point clouds or mesh data in the pre-training dataset. However, explicit autoencoders lack the ability to efficiently exploit the density, as demonstrated in the experiment analysis in Section 4.5 of the main paper. Hence, we consider our approach to have an advantage rather than an unfair comparison.

We also emphasize that we use the same setting as existing self-supervised learning approaches for downstream task training to ensure a fair comparison. Therefore, we are confident that the comparison between our approach and existing approaches is fair.

\section{More Results}
\label{sec:supp:result}

\begin{figure}[t]
    \centering
    \includegraphics[width=\columnwidth]{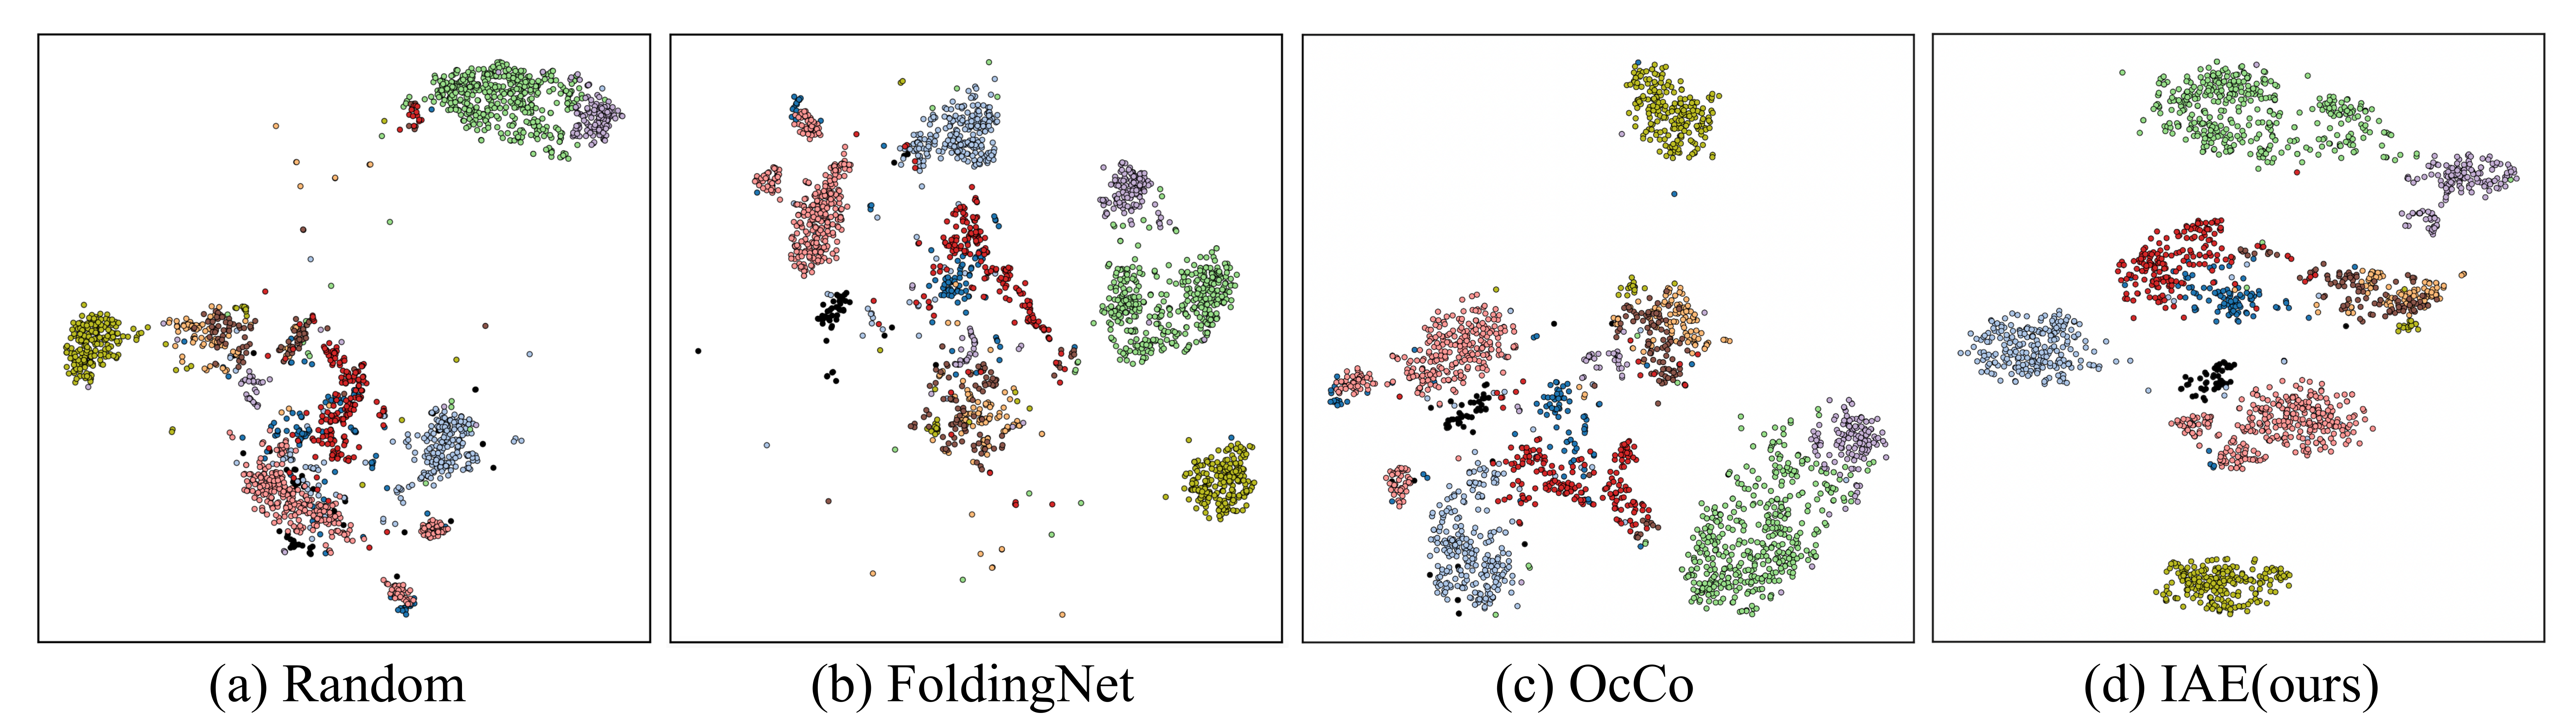}
    \caption{\textbf{Visualization of learned features.} We visualize the learned features for each sample in ModelNet10 using t-SNE. All the models use DGCNN as the encoder backbone. (a) uses random initialization. (b), (c), (d) are pre-trained on ShapeNet.}
    \label{fig:tsne}
    %%\vspace{-2mm}
    %\vspace{-20pt}
\end{figure}

\subsection{Embedding Visualization.} 

We visualize the learned features of our model and baseline approaches in Figure~\ref{fig:tsne}. We compare with FoldingNet~\cite{yang2018foldingnet}, OcCo~\cite{wang2020unsupervised}, and a sanity-check baseline, random initialization. Random initialization use randomly initialized network weights to obtain the embedding, and its performance explains the network prior. The embeddings for different categories in the ModelNet10 dataset are shown using t-SNE dimension reduction. Empirically, we observe that our pre-trained model provides a cleaner separation between different shape categories than FoldingNet~\cite{yang2018foldingnet}, OcCo~\cite{wang2020unsupervised}, and random initialization.

\section{Proof of Propositions}
\label{sec:supp:proof}
Denote 
$$
X = (\bs{x}_1,\cdots, \bs{x}_N),\qquad X'=(\bs{x}_1',\cdots, \bs{x}_N').
$$
To obtain closed-form expressions of the linear auto-encoding problem, we reformulate the optimization problem as 
\begin{equation}
\min\limits_{R, B\in \R^{n\times m}, R^TR = I_m}\ \sum\limits_{k=1}^{N} \|RB^T\bs{x}_k'-\bs{x}_k\|^2
\label{Eq:Opt:Reform}    
\end{equation}

The following proposition specifies the optimal solution to (\ref{Eq:Opt:Reform}).

%\begin{lemma}
The optimal solution $(R^{\star},B^{\star}), R,B\in \R^{n\times m}$ to (\ref{Eq:Opt:Reform}) satisfies that the columns of $R^{\star}$ are the leading $m$ eigenvectors with the largest eigenvalues of 
$$
(X'X)^T(X'{X'}^T)^{+}(X'X^T).
$$
Moreover, 
$$
B^{\star} = (X'{X'}^T)^{+}(X'X^T)R^{\star}.
$$
%\end{lemma}

\begin{proof}
Denote $R = (\bs{r}_1,\cdots, \bs{r}_m)$ and $B = (\bs{b}_1,\cdots, \bs{b}_m)$. Then
\begin{align}
\label{Eq:Obj:Formu}
&\sum\limits_{k=1}^N\|RB^T\bs{x}_k'-\bs{x}_k\|^2 \\
&= \sum\limits_{k=1}^N\Big({\bs{x}_k'}^TBB^T\bs{x}_k' - 2(R^T\bs{x}_k)^T(R^T\bs{x}_k')+\|\bs{x}_k\|^2\Big) \nonumber  \\
&= \sum\limits_{k=1}^{N}\Big(\sum\limits_{j=1}^{m}\big((\bs{b}_j^T\bs{x}_k')^2-2(\bs{r}_j^T\bs{x}_k)(\bs{b}_j^T\bs{x}_k')\big) + \|\bs{x}_k\|^2\Big) \nonumber \\
&= \sum\limits_{j=1}^{m}\Big(\bs{b}_j^T\big(\sum\limits_{k=1}^N\bs{x}_k'{\bs{x}_k'}^T\big)\bs{b}_j - 2(\sum\limits_{k=1}^{N}\bs{x}_k'{\bs{x}_k}^T\bs{r}_j)^T\bs{b}_j\Big) \nonumber \\
& + \sum\limits_{k=1}^{N}\|\bs{x}_k\|^2
\end{align}
Therefore, define
$$
\{\bs{b}_j^{\star},1\leq j \leq m\} = \underset{\bs{b}_j}{\textup{argmin}}\ \sum\limits_{k=1}^{N}\|RB^T\bs{x}_k'-\bs{x}_k\|^2.
$$
Since $\bs{b}_j$ lies in the column space of $X'$, it is clear that the optimal solution $\bs{b}_j^{\star}$ is given by
\begin{align}
\bs{b}_j^{\star} & = \Big(\sum\limits_{k=1}^{N}\bs{x}_k'{\bs{x}_k'}^T\Big)^{+}\Big(\sum\limits_{k=1}^{N}\bs{x}_k'{\bs{x}_k}^T\Big)\bs{r}_j \nonumber \\
&= (X'{X'}^T)^{+}(X'X^T)\bs{r}_j, \qquad 1\leq j \leq m.
\label{Eq:A:Opt}
\end{align}

Substituting (\ref{Eq:A:Opt}) into (\ref{Eq:Obj:Formu}), we have that the objective function becomes
\begin{small}
\begin{align}
&\sum\limits_{k=1}^N\|R{B^{\star}}^T\bs{x}_k'-\bs{x}_k\|^2 \nonumber \\
=&\sum\limits_{j=1}^{m} \bs{r}_j^T\Big(X{X'}^T\Big)\Big(X'{X'}^T\Big)^{+}\Big(X'X^T\Big)\bs{r}_j\nonumber \\
& -2\sum\limits_{j=1}^{m} \bs{q}_j^T\Big(X{X'}^T\Big)^T\Big(X'{X'}^T\Big)^{+}\Big(X'X^T\Big)\bs{r}_j + \sum\limits_{k=1}^{N}\|\bs{x}_k\|^2 \nonumber \\
= &-\sum\limits_{j=1}^{m} \bs{r}_j^T\Big(X'{X}^T\Big)^T\Big(X'{X'}^T\Big)^{+}\Big(X'{X}^T\Big)\bs{r}_j + \sum\limits_{k=1}^{N}\|\bs{x}_k\|^2
\end{align}
\end{small}

Therefore, the optimization problem in (\ref{Eq:Opt:Reform}) reduces to 
\begin{small}
\begin{equation}
\max \limits_{\substack{R\in \R^{n\times m}, \\ R^TR = I_m}} \textup{Trace}\left(R^T \Big(X'{X}^T\Big)^T\Big(X'{X'}^T\Big)^{+}\Big(X'{X}^T\Big) R\right)
\label{Eq:Q:Opt} 
\end{equation}
\end{small}
It is easy to see that the optimal solution $R^{\star} = (\bs{r}_1^{\star},\cdots, \bs{r}_m^{\star})$ to (\ref{Eq:Opt:Reform}) satisfies that $\bs{r}_i^{\star}, i\in [m]$ are the leading $m$ eigenvectors of $C_{X',X}:= \Big(X'{X}^T\Big)^T\Big(X'{X'}^T\Big)^{+}\Big(X'{X}^T\Big)$.
\end{proof}
%Suppose $X' = X + E$. Then it is easy to check that
%\begin{align*}
%\frac{\partial C_{X',X}}{\partial E} = 0.    
%\end{align*}
%In fact, the first-order approximation of $C_{X',X}$ with respect to $E$ is given by
%\begin{align*}
%C_{X',X}  &\approx XX^T+ (EX^T)^T(XX^T)^{-1}(XX^T) + (XX^T)^T(XX^T)^{-1}(EX^T) \nonumber \\
%& \ \ - (XX^T)^T(XX^T)^{-1}(EX^T+XE^T)(XX^T)^{-1}(XX^T) %\nonumber \\
%& = XX^T + XE^T + EX^T - EX^T - XE^T = XX^T.
%\end{align*}

%The implication is that
%$$
%\frac{\partial Q}{\partial E} = 0.
%$$

\subsection{Proof of Proposition 1}

We show that when $\epsilon_k\in \set{L}^{\perp}, k\in [N]$,
$$
R^{\star} = B^{\star} = Q.
$$
Therefore, the formulation of (1) is identical to that of (\ref{Eq:Opt:Reform}). In fact, consider the singular value decomposition (SVD) of 
$$
X' = U\Sigma V^T.
$$
First,
\begin{align*}
X^T X = & X^T X' \\
= & X^TU\Sigma V^T.
\end{align*}
Therefore, $V$ is an orthonormal basis of the column space of $X^T$. This means we can write out the SVD of $X = U'\Sigma'V^T$.
Again using $X^TX = X^T U\Sigma V^T$, we have
$$
V\Sigma'^2 V^T = V \Sigma' {U'}^TU\Sigma V^T.
$$
It follows that
$$
\Sigma'^2 = \Sigma' {U'}^TU\Sigma.
$$
In other words,
$$
U'\Sigma' = U\Sigma.
$$
This means we can arrange the SVD of $X$ so that
$$
U' = U, \Sigma' = \Sigma.
$$

We proceed to show that $(X{X'}^T)(X'{X'}^T)^{+}(X'X^T) = XX^T$. In fact,
\begin{align*}
\ & (X{X'}^T)(X'{X'}^T)^{+}(X'X^T) \\    
= \ & X V\Sigma U^T \big(U\Sigma V^TV\Sigma U^T\big)^{+}(U\Sigma V^T X^T) \\
= \ & X V\Sigma U^T\big(U\Sigma^2 U^T)^{+}(U\Sigma V^T X^T) \\
= \ & X V\Sigma U^TU\Sigma^{-2} U^T U \Sigma V^T X^T \\
= \ & X VV^T X^T \\
= \ & XV\Sigma U^T(U\Sigma^{-2} U^T)U\Sigma V^T X^T \\
= \ & XV\Sigma U^T(U\Sigma^{2} U^T)^{+}U\Sigma V^T X^T \\
= \ & XX^T (XX^T)^{+} XX^T = XX^T.
\end{align*}
Moreover, 
\begin{align*}
\ & (X'{X'}^T)^{+}(X'X^T) \\
=\ & (U\Sigma VV^T\Sigma U^T)^{+} (U\Sigma V^TV\Sigma U) \\
=\ & (U\Sigma^2 U^T)^{+} (U\Sigma^2 U) \\
=\ & I_n. 
\end{align*} 

\qed
%$\square$

\subsection{Proof of Proposition 2}

Let us first consider the case where the corresponding eigenvalues of $Q$ are distinctive. Let $\bs{q}_j, m+1\leq j \leq n$ expand the columns of $Q$ to form an orthonormal basis of $\R^n$. In this case, applying the derivative formula of eigenvectors to each eigenvector and the fact that $\epsilon_k\in \set{L}^{\perp}$, we obtain 
\begin{align}
d\bs{q}_i & = -\sum\limits_{j\neq i}\frac{\bs{q}_j^T\sum\limits_{k=1}^{N}(\bs{x}_k\epsilon_k^T+\epsilon_k\bs{x}_k^T)\bs{q}_i}{\lambda_j-\lambda_i}\bs{q}_j \label{eq:d:q:2} \\
& = -\sum\limits_{j\neq i,j=1}^{m}\frac{\bs{q}_j^T\sum\limits_{k=1}^{N}(\bs{x}_k\epsilon_k^T+\epsilon_k\bs{x}_k^T)\bs{q}_i}{\lambda_j-\lambda_i}\bs{q}_j\\ & \quad -\sum\limits_{j=m+1}^{n}\frac{\bs{q}_j^T\sum\limits_{k=1}^{N}(\bs{x}_k\epsilon_k^T+\epsilon_k\bs{x}_k^T)\bs{q}_i}{\lambda_j-\lambda_i}\bs{u}_j \nonumber \\
& = -\sum\limits_{j=m+1}^{n}\frac{\bs{q}_j^T\sum\limits_{k=1}^{N}\epsilon_k\bs{x}_k^T\bs{q}_i}{\lambda_j-\lambda_i}\bs{q}_j \nonumber \\
& =\big(\sum\limits_{j=m+1}^{n}\bs{q}_j\bs{q}_j^T\big)\big(\sum\limits_{k=1}^{N}\epsilon_k \bs{x}_k^T\big) \bs{q}_i\lambda_i^{-1} \\
&= \big(I_n-QQ^T\big)\sum\limits_{k=1}^{N}\epsilon_k \bs{x}_k^T \bs{q}_i\lambda_i^{-1}.
\label{Eq:d:q:formula}
\end{align}
It is easy to check that 
\begin{align*}
d\bs{q}_i^T\bs{q}_i = 0 & \qquad 1\leq i \leq m \\
d\bs{q}_i^T\bs{q}_j + d\bs{q}_j^T\bs{q}_i = 0 &\qquad  1\leq i\neq j \leq m
\end{align*}
Therefore, $Q^T\hat{Q}^{\star} \approx I_2$ up to second-order errors $O(\{\|\epsilon_k^2\|\})$. Therefore, the rotation matrix used to calibrate $\hat{Q}^{\star}$ and $Q$ when defining $\mathcal{D}(\hat{Q}^{\star}, Q)$ is the identity matrix up to second-order errors $O(\{\|\epsilon_k^2\|\})$. Applying (\ref{Eq:d:q:formula}), we have
\begin{align*}
& \quad \frac{\partial \set{D}(\hat{Q}^{\star}, Q)}{\partial \epsilon_{ki}} \\
& = \big(I_n-QQ^T\big) \left(\bs{e}_k\bs{x}_k^T\bs{q}_1\lambda_1^{-1},\cdots,\bs{e}_k\bs{x}_k^T\bs{q}_m\lambda_m^{-1}\right) \\
& = (I_n-QQ^T)\bs{e}_k \bs{x}_k^T Q\Lambda^{-1}.
\end{align*}
The proof under the case where the eigenvalues of $Q$ are repeating is similar, except that the summation in (\ref{eq:d:q:2}) shall discard $(i,j)$ pairs where $\lambda_i = \lambda_j$. On the other hand, the uncertainties in eigenvectors when having repeating eigenvalues are addressed by the calibration rotation matrix in $\mathcal{D}(\hat{Q}^{\star},Q)$.

\qed
