# Supplementary material for: Implicit Autoencoder for Point-Cloud Self-Supervised Representation Learning
Source: arXiv:2201.00785 source file (2023-08-27)
Supplement: Supplementary file 2 [file supp_compare.tex]

\begin{figure}[t]
    \centering
    \includegraphics[width=\columnwidth]{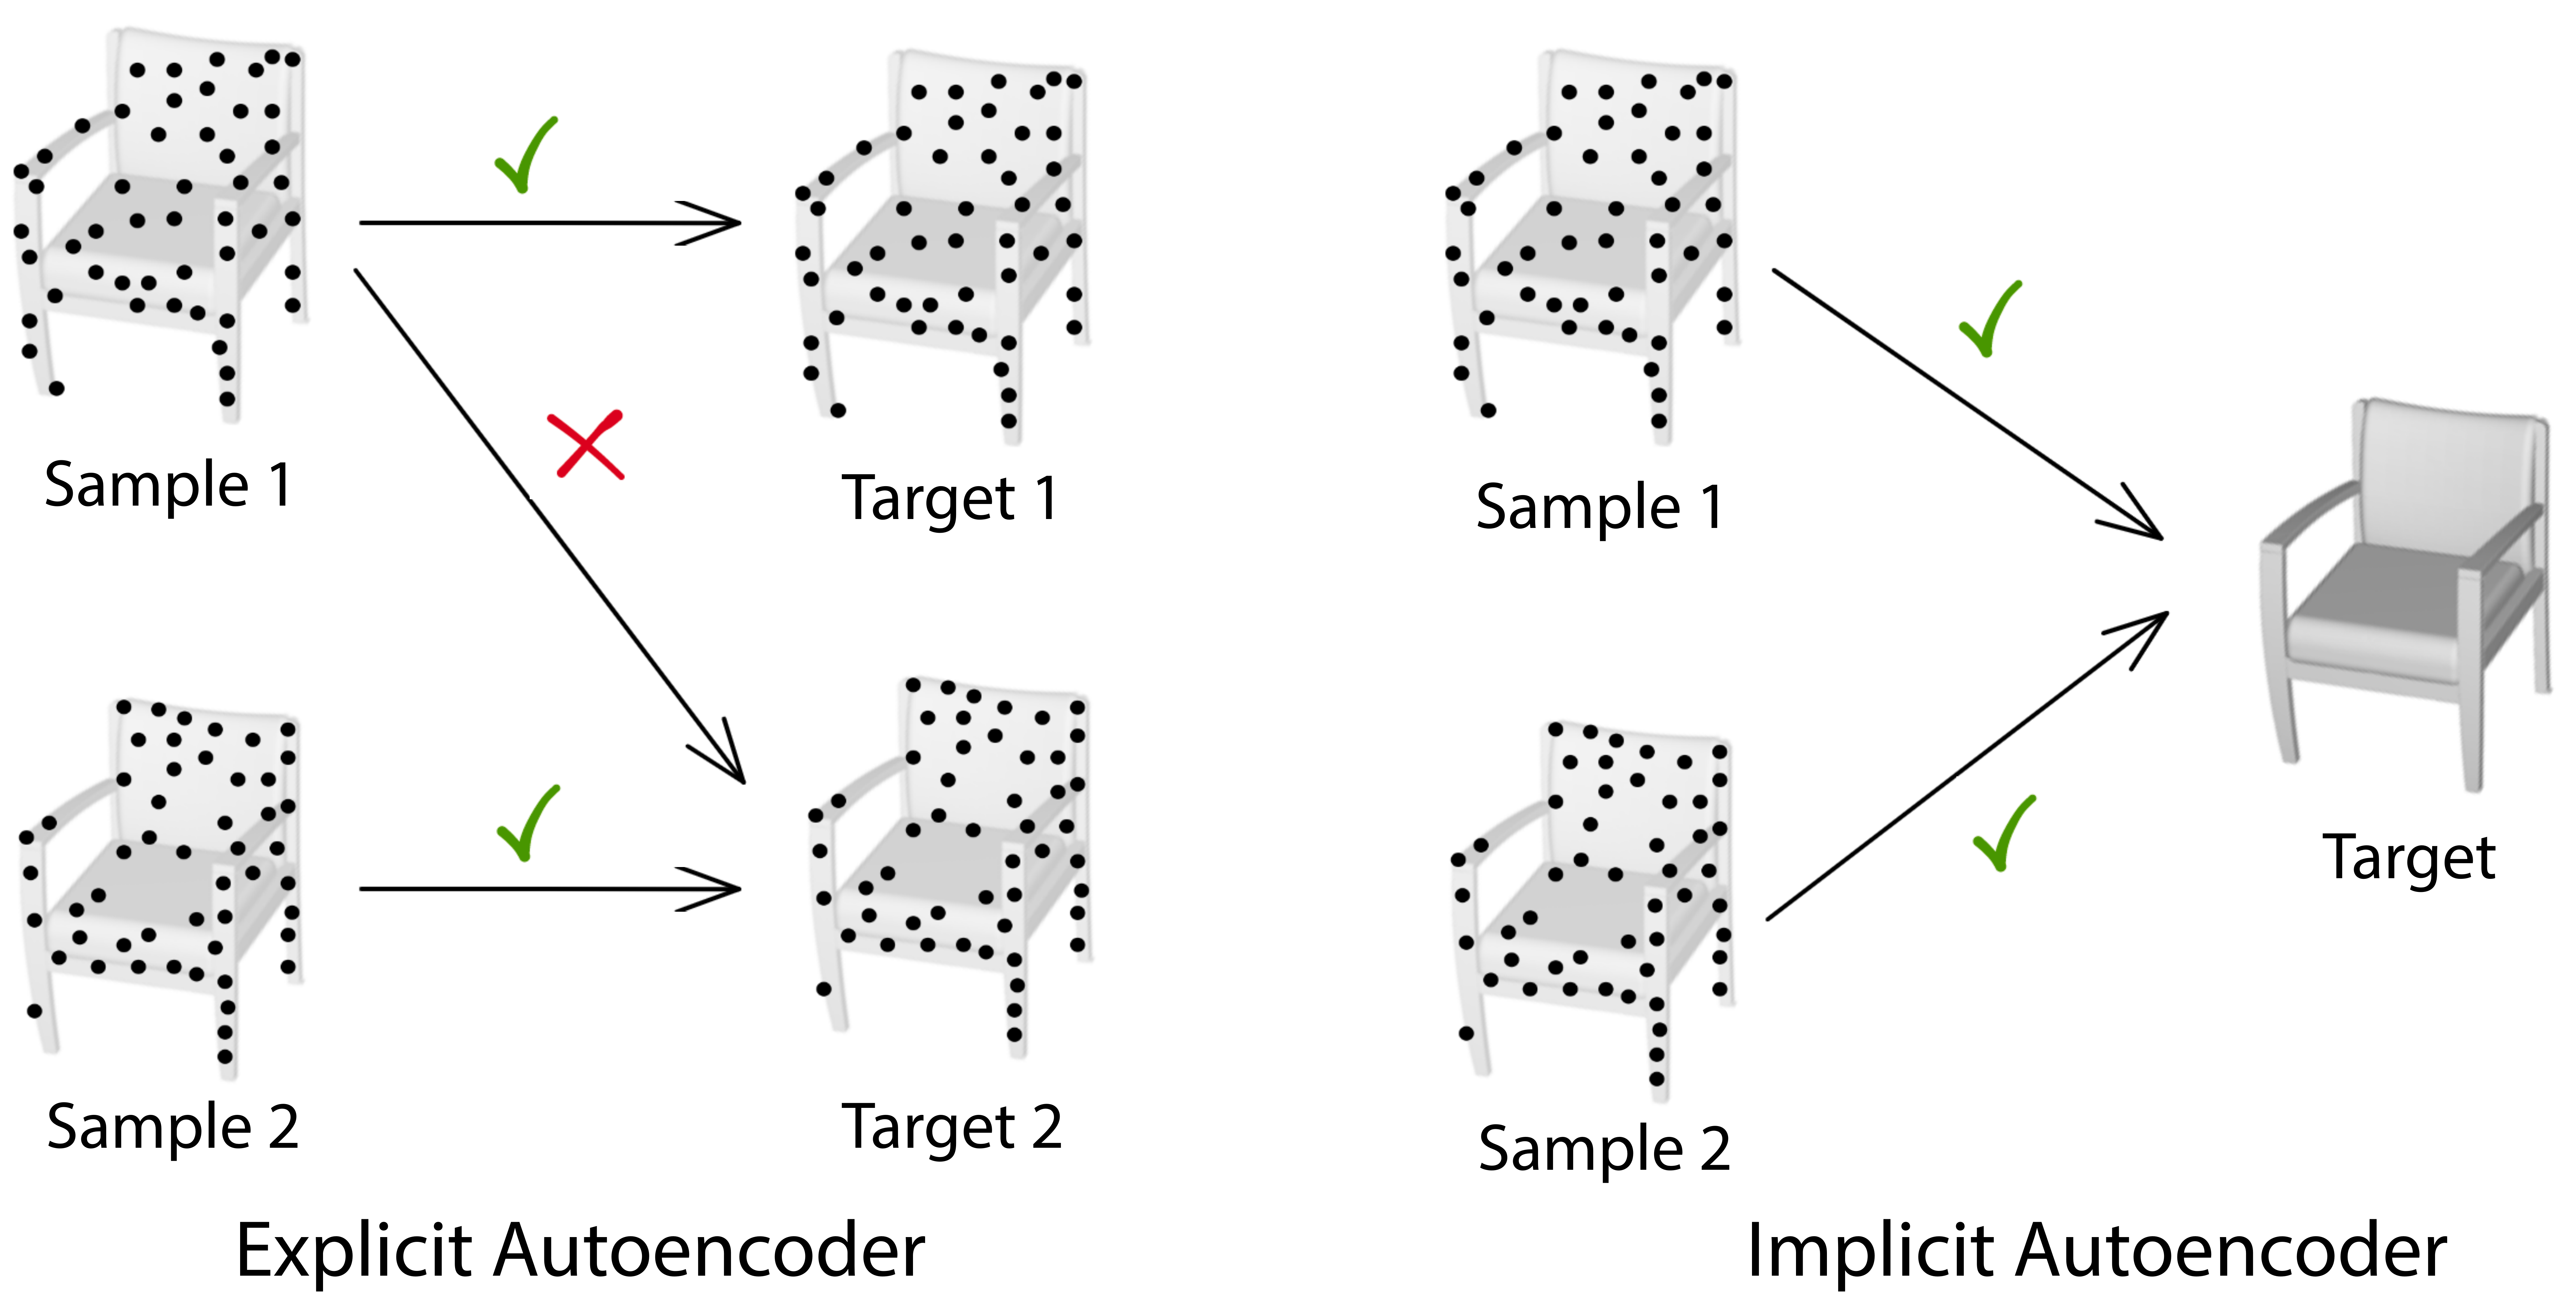}
    \caption{\small{\textbf{Comparison between Explicit Autoencoder and Implicit Autoencoder}. Given a 3D shape, we randomly take two samples. For Implicit Autoencoder, we use 3D CAD model to represent the implicit function target for better visualization.}}
    \label{fig:supp_compare}
    \vspace{-10pt}
\end{figure}
